# Supplementary material for: Autoencoding Undirected Molecular Graphs With Neural Networks
Source: arXiv:2001.03517 source file (2020-03-21)
Supplement: Supplementary file 1 [file main_SI.tex]

\documentclass{report}
\usepackage[utf8]{inputenc}
\usepackage{graphicx}
\usepackage{amsmath,graphicx}
\usepackage{amssymb}
\usepackage[T1]{fontenc}  % thanks's daleif
\usepackage[utf8]{inputenc}
\usepackage[english]{babel}
\usepackage{lipsum}
\usepackage{subfiles}
\usepackage{siunitx}
\usepackage{multirow}
\usepackage{caption}
\usepackage{subcaption}
\usepackage{float}
\title{Supporting information for Autoencoding undirected molecular graphs with neural networks}

\author{Jeppe Johan Waarkjær Olsen \and Peter Ebert Christensen \and
Martin Hangaard Hansen \and Alexander Rosenberg Johansen}
%\date{November 2019}
%\renewcommand{\figurename}{Figure S}

\begin{document}

\maketitle

\input{SI/si.tex}
\input{SI/qm9.tex}
\input{SI/zinc.tex}
\end{document}
